# Supplementary material for: Efficient Semantic Segmentation using Gradual Grouping
Source: arXiv:1806.08522 source file (2018-06-22)
Supplement: Supplementary file 1 [file appendix.tex]

\appendix
This appendix provides formal proofs for the theorems stated in Section 3 of the main paper. We also include tabulation of results of Figure 3 and 4, alongside additional results that could not be added in the paper due to space constraints.

\section{Explicit Expanders}
In this section, we will give details about some properties of expander graphs that are required for proving Theorems 1 and 2. Expander graphs are characterized by the spectral gap, which in turn implies the connectivity properties listed in Section 3.1. Many constructions of expander graphs have been explored in the past (see \cite{expsurvey}). We will be using a construction that is comparatively easy to describe and implement. We will be considering Cayley graphs, which are obtained from the theory of finite Fields/Groups. The vertex set of such graphs is a group and the edges are defined by addition operation on the vertices. Also we will be describing expanders that are simple undirected graphs. Given an undirected graph $G=(V,E)$, we can obtain  a bipartite expander $G=(V,V',E)$, by making a copy of the vertices $V$ on the other side and adding edges according to $E$.

\subsection{Cayley Expander}
Let $V$ be a group under an operation $+$ and let $H \subset V$ be a set of generators of the group $V$. The Cayley graph defined by $V,H$ is the graph with vertex set $V$ and the edges $E =\{(x,x+h) : h \in H\}$. For our construction, we will consider the group $\{0,1\}^n$ under coordinate-wise XOR operations. For $H \subset \{0,1\}^n$, the Cayley graph defined by $H$ is $|H|$-regular. It is a well-known result in spectral graph theory that there are set of generators $H$, for which the Cayley graph defined by $\{0,1\}^n, H$ forms an expander with spectral gap $\gamma$.
\begin{theorem*}[Alon, Roichman, Proposition 4 \cite{cayley}]
For every $\epsilon$,  there exists explicit $H \subset \{0,1\}^n$ of size $\leq O(n^2/\epsilon^2)$ such that the Cayley graph defined by $\{0,1\}^n, H$ is an expander with spectral gap $\gamma = 1-\epsilon$.
\end{theorem*}

The properties given in Section 3.1 follows from the fact that expanders have a spectral gap (for proofs see \cite{pseudo}). For the sensitivity proofs, we need the following lemmas. The first lemma states that having a spectral gap, implies that all set of vertices of size $\leq n/2$ expands.
\begin{lemma}[Theorem 4.6 \cite{pseudo}] 
\label{lab:spec}
If $G=(V,E)$ is an expander with spectral gap of $\gamma$ then for every subset $S\subset V$ of size $\leq |V|/2$, the size of the set of neighbors $|N(S)| \geq (1+\gamma) |S|$.
\end{lemma}
The next lemma is known as the expander mixing lemma, deals with the uniform connectivity properties of the expander.
\begin{lemma}[Lemma 4.15 \cite{pseudo}]
\label{lab:exp-mix-lem}
If $G=(V,E)$ is an $D$-regular expander with spectral gap of $\gamma$ then for every subset $S,T\subset V$,
$$\left| E(S,T) - D \cdot |S| \cdot |T| / n  \right| \leq (1-\gamma)\sqrt{|S| \cdot |T|}$$
where $E(S,T)$ is the set of edges from $S$ to $T$.
\end{lemma}

\section{Sensitivity in Expanders}
In this section, we prove Theorem 1 and Theorem 2 using the properties described above along with the connectivity properties defined in Section 3.1 of the paper.
\begin{theorem}[Sensitivity of X-Nets]\label{thm:conn}
Let $n$ be the number of input as well as output nodes in the network and $G_1,G_2,\cdots, G_t$ be $D$ regular bipartite expander graphs with $n$ nodes on both sides. Then  
every output neuron is sensitive to every input in a Deep X-Linear Network defined by $G_i$'s with depth $t = O( \log n)$.
\end{theorem}
\begin{proof}
For showing sensitivity, we show that for every pair of input and output $(u,v)$,  there is a path in the X-Net with the $i^{th}$ edge from the $i^{th}$ graph. 
We use the expansion property of the expander graphs. Let $N_1(u)$ be the set of neighbors of $u$ in $G_1$ and $N_i(u)$ be the set of neighbors of $N_{i-1}(u)$ in the graph $G_i$. Since each of the graphs are expanding $|N_{i}(u)| \geq (1+\gamma) \times |N_{i-1}(u)|$, using Lemma \ref{lab:spec}. Since $(1+\gamma) > 1$, we can obtain that for $i = O(\log n)$, $|N_i(u)| \geq n/2$. Similarly we can start from $v$ and define $N_1(v)$ as the set of neighbors of $v$ in $G_t$ and $N_i(v)$ be the set of neighbors of $N_{i-1}(v)$ in the graph $G_{n-i -1}$. Due to the expansion property, for $j = O(\log n)$, $|N_j(v)| \geq n/2$. Now we choose $t = i + j = O(\log n)$ so that the $i^{th}$ graph from $1$ is the same as $j+1^{th}$ graph from $t$. Then we will have that $N_i(u) \cap N_j(v) \neq \phi$. That is there is some vertex in the $i^{th}$ graph that is both connected to $u$ and $v$, which implies that there is a path from $u$ to $v$.
\end{proof}

\begin{theorem}[Mixing in Deep Expander Networks]
Let $n$ be the number of input as well as output nodes in the network and $G_1,G_2,\cdots, G_t$ be $D$ regular bipartite expander graphs with $n$ nodes on both sides. Let $S,T$ be subsets of input and output nodes in the X-Linear Network defined by the $G_i$'s. The number of paths between $S$ and $T$ is $\approx D|S||T|/n$
\end{theorem}
\begin{proof}
First we prove the theorem for the case when $G_1 = G_2 \cdots = G_t = G$. Note that for $t=1$, the theorem is same as the expander mixing lemma (Lemma \ref{lab:exp-mix-lem}). For $t>1$, consider the graph of $t$ length paths denoted by $G^t$. An edge in this graph denotes that there is a path of length $t$ in $G$. Observe that the adjacency matrix of $G^t$ is given by the $t$th power of the adjacency matrix of $G$ and hence the spectral gap of $G^t$, $\gamma_t = \gamma^t$. Now applying the expander mixing lemma on $G^t$ (Lemma \ref{lab:exp-mix-lem}), proves the theorem.

For the case when the graph $G_i$'s are different, let $\gamma_{\min}$ be the minimal spectral gap among the graphs. Since all the graphs are $D$-regular, the largest eigenvector is the all ones vector with eigenvalue $D$ for all the graphs. The eigenvector corresponding to second largest eigenvalue can be different for each graph, but they are orthogonal to the all ones vector. Hence the spectral gap of the $t$ length path graph $G$ is at least $\gamma_{\min}^t$. Finally we apply the expander mixing lemma on $G^t$ to prove the theorem.
\end{proof}

\section{Model Details}

\begin{table}[t]
\resizebox{\columnwidth}{!}{
\begin{tabular}{|l|c|c|c|}
\hline
{\bf AlexNet} & {\bf Filter Shape} & {\bf Filter Shape} & {\bf Filter Shape} \\
\hline
 &  & ({\bf X-AlexNet-1}) & ({\bf X-AlexNet-2})\\
 \hline
Conv2d & 64 x 3 x 11 x 11 & 64 x 3 x 11 x 11 & 64 x 3 x 11 x 11\\
Conv2d & 192 x 64 x 5 x 5 & 192 x 64 x 5 x 5 & 192 x 64 x 5 x 5\\
Conv2d & 384 x 192 x 3 x 3 & 384 x 192 x 3 x 3 & 384 x 192 x 3 x 3\\
Conv2d & 256 x 384 x 3 x 3 & 256 x 384 x 3 x 3 & 256 x 384 x 3 x 3\\
Conv2d & 256 x 256 x 3 x 3 & 256 x 256 x 3 x 3 & 256 x 256 x 3 x 3\\
\hline
Linear & 9216 x 4096 & 1024 x 4096 & 512 x 4096\\
Linear & 4096 x 4096 & 512 x 4096 & 512 x 4096\\
Linear & 4096 x 1000 & 1024 x 1000 & 1024 x 1000\\
\hline
\end{tabular}}
\vspace{0.1cm}
\caption{Filter sizes for the AlexNet model. Notice the filter sizes of the linear layers of the original model has $|V|\times |U|$ parameters, whereas X-AlexNet models have $|V|\times D$ parameters. Note that $D << |U|$ as stated in Section 3.2. Hence, expander graphs model connections in linear layers (X-Linear) effectively.}
\label{tab:vgg}
\end{table}
\begin{table}[t]
\resizebox{\columnwidth}{!}{
\begin{tabular}{|l|c|c|c|}
\hline
{\bf VGG} & {\bf Filter Shape} & {\bf Filter Shape} & {\bf Filter Shape}\\
\hline
 &  & ({\bf X-VGG16-1}) & ({\bf X-VGG16-2})\\
 \hline
Conv2d & 64 x 3 x 3 x 3 & 64 x 3 x 3 x 3 & 64 x 3 x 3 x 3\\
Conv2d & 64 x 64 x 3 x 3 & 64 x 64 x 3 x 3 & 64 x 64 x 3 x 3\\
Conv2d & 128 x 64 x 3 x 3 & 128 x 64 x 3 x 3 & 128 x 64 x 3 x 3\\
Conv2d & 128 x 128 x 3 x 3 & 128 x 64 x 3 x 3 & 128 x 64 x 3 x 3\\
Conv2d & 256 x 128 x 3 x 3 & 256 x 32 x 3 x 3 & 256 x 16 x 3 x 3\\
Conv2d & 256 x 256 x 3 x 3 & 256 x 32 x 3 x 3 & 256 x 16 x 3 x 3\\
Conv2d & 256 x 256 x 3 x 3 & 256 x 32 x 3 x 3 & 256 x 16 x 3 x 3\\
Conv2d & 512 x 256 x 3 x 3 & 512 x 32 x 3 x 3 & 512 x 16 x 3 x 3\\
Conv2d & 512 x 512 x 3 x 3 & 512 x 32 x 3 x 3 & 512 x 16 x 3 x 3\\
Conv2d & 512 x 512 x 3 x 3 & 512 x 32 x 3 x 3 & 512 x 16 x 3 x 3\\
Conv2d & 512 x 512 x 3 x 3 & 512 x 32 x 3 x 3 & 512 x 16 x 3 x 3\\
Conv2d & 512 x 512 x 3 x 3 & 512 x 32 x 3 x 3 & 512 x 16 x 3 x 3\\
Conv2d & 512 x 512 x 3 x 3 & 512 x 32 x 3 x 3 & 512 x 16 x 3 x 3\\
\hline
Linear & 512 x 512 & 128 x 512 & 128 x 512\\
Linear & 512 x 10 & 512 x 10 & 512 x 10\\
\hline
\end{tabular}}
\vspace{0.1cm}
\caption{Filter sizes for the VGG-16 model on CIFAR-10 dataset. The filter sizes given are $|V|\times |U| \times c \times c$ in original VGG network, $|V|\times D \times c \times c$ in our X-VGG16 models. Note that $D << |U|$ as stated in Section 3.2. Hence, expander graphs model connections in Convolutional layers (X-Conv) effectively.}
\label{tab:alexnet}
\end{table}

We discuss the model structures in detail, along with tabulated  values of size and flops of various architectures presented as graphs in the main paper in Figure 3 and 4. 
\begin{table}[t]
\resizebox{\columnwidth}{!}{
\begin{tabular}{|l|c|c|c|}
\hline
{\bf Model} & {\bf Accuracy} & {\bf \#Params } & {\bf \#FLOPs}\\
\hline
CIFAR10 &  & {\bf(in M)} & {\bf(in 100M)}\\
\hline
X-DenseNetBC-2-40-24 & {\bf 94.83\%} & {\bf 0.4M} & {\bf 1.44}\\
DenseNetBC-40-24 & 94.79\% & 0.7M & 2.88\\
X-DenseNetBC-2-40-36 & 94.98\% & 0.75M & 3.24\\
X-DenseNetBC-2-40-48 & {\bf 95.48\%} & {\bf 1.4M} & {\bf 5.75}\\
DenseNetBC-40-36 & 95.26\% & 1.5M & 6.47\\
X-DenseNetBC-2-40-60 & {\bf 95.71\%} & {\bf 2.15M} & {\bf 8.98}\\
DenseNetBC-40-48 & 95.64\% & 2.8M & 11.50\\
DenseNetBC-40-60 & 95.91\% & 4.3M & 17.96\\
\hline
CIFAR100 &  &  &\\
\hline
X-DenseNetBC-2-40-24 & 74.37\% & 0.4M & 1.44\\
DenseNetBC-40-24 & 76.05\% & 0.7M & 2.88\\
X-DenseNetBC-2-40-36 & {\bf 76.69\%} & {\bf 0.75M} & {\bf 3.24}\\
DenseNetBC-40-36 & 77.84\% & 1.5M & 6.47\\
X-DenseNetBC-2-40-60 & 78.53\% & 2.15M & 8.98\\
X-DenseNetBC-4-70-60 & {\bf 79.56\%} & {\bf 2.6M} & {\bf 10.26}\\
DenseNetBC-40-48 & 79.03\% & 2.8M & 11.50\\
DenseNetBC-40-60 & 79.87\% & 4.3M & 17.96\\
X-DenseNetBC-2-70-60 & 80.89\% & 5.18M & 20.52\\
DenseNetBC-70-60 & 81.28\% & 10.36M & 41.05\\
\hline
\end{tabular}}
\vspace{0.1cm}
\caption{Results obtained on the state-of-the-art models on CIFAR-10 and CIFAR-100 datasets, ordered by FLOPs per model. X-Nets give significantly better accuracies with corresponding DenseNet models in the same limited computational budget and correspondingly significant parameter and FLOP reduction for models with similar accuracy.}
\label{tab:cifar}
\end{table}
\subsection{Filter structure of AlexNet and VGG}

In Tables \ref{tab:vgg} and \ref{tab:alexnet}, the detailed layer-wise filter structure is tabulated as stated in Section 5.2 of the paper. We compare the sizes of input channels between the filters, and show that with X-Conv and X-Linear layers, we can train models effectively even with upto 32x and 18x times smaller filters in input dimension in VGG16 and AlexNet models respectively. Hence, modeling connections as weighted adjacency matrix of an Expander graph is an effective method to model connections between neurons, producing highly efficient X-Nets.

\subsection{Results}
As stated in Section 5.2, Tables \ref{tab:cifar} and \ref{tab:imagenet} presented below give the detailed accuracy, parameters and FLOPs of models displayed in the Figure 3 in the paper. Details of other models are also provided in the same table, which could not be displayed in the paper due to lack of space.

Table \ref{tab:cifar} displays the performance of X-DenseNet models on the CIFAR-10 and CIFAR-100 datasets. If we compare models that have similar number of parameters, we achieve around 0.2\% and 0.6\% increase in accuracy over DenseNet-BC models on CIFAR-10 and CIFAR-100 datasets respectively. In the same manner, we can achieve upto using only two-thirds of the parameter and runtime cost cost respectively, keeping accuracy constant on CIFAR-10 and CIFAR-100 datasets as stated in the paper.

\begin{table}[t]
\resizebox{\columnwidth}{!}{
\begin{tabular}{|l|c|c|c|}
\hline
{\bf Model} & {\bf Accuracy} & {\bf \#Params } & {\bf \#FLOPs}\\
\hline
ResNet &  & {\bf(in M)} & {\bf(in 100M)}\\
\hline
X-ResNet-2-34 & 69.23\% & 11M & 35\\
X-ResNet-2-50 & {\bf 72.85\%} & {\bf 13M} & {\bf 40}\\
ResNet-34 & 71.66\% & 22M & 70\\
X-ResNet-2-101 & {\bf 74.87\%} & {\bf 22.5M} & {\bf 80}\\
ResNet-50 & 74.46\% & 26M & 80\\
ResNet-101 & 75.87\% & 45M & 160\\
\hline
DenseNetBC &  &  & \\
\hline
MobileNet \cite{howard2017mobilenets} & 70.6\% & 4.2M & 5.7 \footnote{These are reported as mult-add operations} \\
ShuffleNet \cite{zhang2017shufflenet} & 70.9\% & 5M & 5.3 \footnote{These are reported as mult-add operations} \\
X-DenseNetBC-2-121 & {\bf 70.5\%} & {\bf 4M} & 28\\
X-DenseNetBC-2-169 & 71.7\% & 7M & 33\\
X-DenseNetBC-2-201 & 72.5\% & 10M & 43\\
X-DenseNetBC-2-161 & {\bf 74.3\%} & 14.3M & {\bf 55}\\
DenseNetBC-121 & 73.3\% & 8M & 55\\
DenseNetBC-169 & 74.8\% & 14M & 65\\
DenseNetBC-201 & 75.6\% & 20M & 85\\
DenseNetBC-161 & 76.3\% & 28.5M & 110\\
\hline
\end{tabular}}
\vspace{0.1cm}
\caption{Results obtained on the state-of-the-art models on ImageNet dataset, ordered by FLOPs. We also observe that X-DenseNetBC models outperform ResNet and X-ResNet models in both compression, parameters and FLOPs and achieve comparable accuracies with the highly efficient MobileNets and ShuffleNets in the same parameter budget, albeit with much higher FLOPs due to architectural constraints.}
\label{tab:imagenet}
\end{table}

Similarly, Table \ref{tab:imagenet} displays the performance of X-ResNet and X-DenseNet models on the ImageNet datasets. We can observe that we achieve around 3.2\% and 1\% increase in accuracy over ResNet and DenseNet-BC models in the same computational budget. Also, we can observe that we require approximately 15\% less FLOPs for achieving similar accuracies over DenseNet models and 15\% less parameters for achieving similar accuracies over the ResNet model respectively as stated in the paper. We also observe that X-DenseNetBC models outperform ResNet and X-ResNet models in both compression, parameters and FLOPs and achieve comparable accuracies with MobileNets \cite{howard2017mobilenets} and ShuffleNets \cite{zhang2017shufflenet} in the same parameter budget, albeit with much higher computational cost due to architectural constraints. 

\begin{table}[t]
\resizebox{\columnwidth}{!}{
\begin{tabular}{|l|c|c|c|}
\hline
{\bf Model} & {\bf Accuracy} & {\bf \#Params } & {\bf \#FLOPs}\\
\hline
Wider & & {\bf(in M)} & {\bf(in 100M)} \\
\hline
DenseNetBC-40-60 & 79.87\% & 4.3M & 17.96\\
X-DenseNetBC-2-40-60 & 78.53\% & 2.15M & 8.98\\
X-DenseNetBC-4-40-60 & 77.54\% & 1.08M & 4.49\\
X-DenseNetBC-8-40-60 & 75.29\% & 0.54M & 2.24\\
X-DenseNetBC-16-40-60 & 74.44\% & 0.27M & 1.12\\
\hline
DenseNetBC-40-100 & 80.9\% & 11.85M & 49.85\\
X-DenseNetBC-4-40-100 & 78.87\% & 2.9M & 12.46\\
X-DenseNetBC-8-40-100 & 77.75\% & 1.48M & 6.23\\
X-DenseNetBC-16-40-100 & 76.2\% & 0.74M & 3.12\\
\hline
DenseNetBC-40-200 & 81.62\% & 47.19M & 199.28\\
X-DenseNetBC-4-40-200 & 80.66\% & 11.79M & 49.82\\
X-DenseNetBC-10-40-200 & 79.46\% & 4.71M & 19.93\\
X-DenseNetBC-20-40-200 & 78.33\% & 2.3M & 9.96\\
X-DenseNetBC-30-40-200 & 77.29\% & 1.6M & 6.64\\
X-DenseNetBC-50-40-200 & 75.7\% & 0.9M & 3.99\\
X-DenseNetBC-80-40-200 & 73.26\% & 0.5M & 2.49\\
\hline
Deeper &  &  &\\
\hline
DenseNetBC-40-60 & 79.87\% & 4.3M & 17.96\\
X-DenseNetBC-2-40-60 & 78.53\% & 2.15M & 8.98\\
X-DenseNetBC-8-40-60 & 77.54\% & 0.54M & 2.24\\
X-DenseNetBC-16-40-60 & 75.29\% & 0.27M & 1.12\\
\hline
DenseNetBC-58-60 & 80.79\% & 7.66M & 30.96\\
X-DenseNetBC-2-58-60 & 80.29\% & 3.83M & 15.48\\
X-DenseNetBC-4-58-60 & 78.74\% & 1.9M & 7.74\\
X-DenseNetBC-8-58-60 & 77.98\% & 0.95M & 3.87\\
X-DenseNetBC-16-58-60 & 75.87\% & 0.47M & 1.93\\
\hline
DenseNetBC-70-60 & 81.28\% & 10.36M & 41.05\\
X-DenseNetBC-2-70-60 & 80.89\% & 5.18M & 20.52\\
X-DenseNetBC-4-70-60 & 79.56\% & 2.6M & 10.26\\
X-DenseNetBC-8-70-60 & 77.48\% & 1.3M & 5.13\\
X-DenseNetBC-16-70-60 & 77.23\% & 0.65M & 2.57\\
\hline
\end{tabular}}
\vspace{0.1cm}
\caption{We display accuracies, parameters and FLOPs of all the wider and deeper networks on CIFAR-100 listed in increasing compression order. This proves that efficiently designing layers like X-Conv and X-Linear allows us to train wider and deeper networks frugally.}
\label{tab:ultranets}
\end{table}

Table \ref{tab:ultranets} displays accuracies, parameters and FLOPs of all the wider and deeper networks trained on CIFAR-100 dataset as discussed in Section 5.7. They are listed in increasing compression order from DensenetBC (1x) to the highest compressed X-DenseNet. The figure indicates that Expander Graphs modeling can scale up to high compression ratios without drastic drops in accuracies, enabling us to train deeper and wider networks retaining similar FLOPs and parameters effectively. We believe this modeling can open up a interesting exploration of training significantly deeper and wider range of models, unlike the current compression techniques as X-Nets are highly compressed networks since definition. 

\subsubsection{Additional Training Details}
All models in the plot were trained from the ImageNet code available on Pytorch Official repository including the original DenseNet and ResNet models. Note that this training code is common for all models in the repository and not fine-tuned to any specific model like ResNet or DenseNet. Hence the accuracies we report is slightly lower that those reported using model-specific training code. However, note that we have used the same code for training both the original models and the expander versions of these models. Hence the comparison is a fair one. Same is true with the  AlexNet model. Note that we use the original AlexNet architecture, and not CaffeNet. 
In contrast, training with fine-tuned code is expected to give a 1-2\% improvement over MobileNets in Table \ref{tab:imagenet}. Training schedules suited to X-Nets, hyper-parameter tuning, Activation layers tailored to X-Nets could further improve the accuracies. Overall, we believe that investigating training methods for X-Nets has a lot of potential for improving their performance.
